# Supplementary material for: Bosonic Condensation and Disorder-Induced Localization in a Flat Band
Source: arXiv:1505.05652 ancillary file (2016-02-17)
Supplement: Supplementary file 1 [file Supplemental_Material.pdf]

# Supplemental Material for: "Bosonic Condensation and Disorder-Induced Localization in a Flat Band"

F. Baboux,[1] L. Ge,[2,3] T. Jacqmin,[1,*] M. Biondi,[4] E. Galopin,[1] A. Lemaître,[1] L. Le Gratiet,[1] I. Sagnes,[1] S. Schmidt,[4] H. E. Türeci,[5] A. Amo,[1] and J. Bloch[1]

[1]*Laboratoire de Photonique et Nanostructures, LPN/CNRS, Route de Nozay, 91460 Marcoussis, France*
[2]*Department of Engineering Science and Physics, College of Staten Island, CUNY, New York 10314, USA*
[3]*The Graduate Center, CUNY, New York 10016, USA*
[4]*Institute for Theoretical Physics, ETH Zurich, 8093 Zurich, Switzerland*
[5]*Department of Electrical Engineering, Princeton University, Princeton, New Jersey 08544, USA*

**Contents**

I. METHODS 1
A. Interferometric measurements 1
B. Tight-binding parameters of the 1D Lieb lattice 2
C. Calculation of the condensation modes 2
D. Calculation of the participation ratio 3

II. SUPPLEMENTARY EXPERIMENTAL DATA AND ANALYSIS 4
A. Condensation process 4
1. Band structure versus pump power 4
2. Emission intensity and linewidth versus pump power 6
B. Properties of the condensates 6
1. Spatial map of the emission energy 7
2. Phase structure of the condensates 7
3. Estimation of disorder strength in our samples 8
4. Effect of diagonal Vs. non-diagonal disorder in the flat band 8
5. Estimation of polariton-polariton interactions 9
6. Stability of flat band condensates 10

References 11

## I. METHODS

### A Interferometric measurements

To probe the spatial coherence in the condensation regime (Fig. 3a-f of the main text), we use standard interferometric techniques[1]. We split the sample emission into the two arms of a Michelson interferometer. Both arms contain an identical image of the condensate, except that in one arm we shift the image by an amount $\Delta x$ along the periodic direction. Then both image

recombine on the CCD camera, so that each point $(x, y)$ (coordinates along the periodic direction and perpendicular to it, respectively) of the emission interferes with the point located at $(x+\Delta x, y)$. This produces an interference pattern, whose visibility at each point $(x, y)$ equals the first-order spatial coherence $g^{(1)}((x, y); (x + \Delta x, y))$. By averaging on $x$ and $y$ over the interferogram, we obtain the mean spatial coherence $g^{(1)}(\Delta x)$, which is the quantity plotted in Fig. 3g of the main text. Note that we use a low-pass filter to suppress the scattered pump beam, so that is does not participate in the observed interference.

When $\Delta x$ is modified (see e.g. Figs. 3a to 3c), the relative angle between the two images incident on the CCD camera changes slightly, and thus the orientation and spatial period of the fringes change accordingly. However, this does not modify the visibility of the fringes, which is the only parameter relevant for determining the coherence length. Note also that for a given $\Delta x$ the fringe structure is identical for both types of condensates (flat and dispersive band).

### B Tight-binding parameters of the 1D Lieb lattice

The parameters of the lattice Hamiltonian $\mathcal{H}_{\mathrm{Lieb}}$ (see main text) reproducing the band structure in the low power regime (Figs. 2b,h) are the following. For TM polarization (Fig. 2b) we used $t_1 = 0.17$ meV, $t_2 = 0.22$ meV and $t' = -0.04$ meV. The on-site energies of pillars A and C are identical ($E_A = E_C$), and that of pillars B is slightly redshifted ($E_B = E_A - 0.15$ meV) to account for the fact that these pillars have the maximum number of neighbors and hence a reduced confinement energy.

For TE polarization (Fig. 2h) we used the same parameters, except for a rigid blueshift 0.07 meV of all pillars and an additional blueshift 0.18 meV of sites C; these blueshifts account for the polarization anisotropy of the structure (due to polarization-dependent boundary conditions).

The couplings between pillars can be experimentally adjusted by changing the distance between pillars, or alternatively by changing the exciton-photon detuning (a larger photonic fraction of polaritons will result in higher tunnel couplings). Here, these parameters have been chosen so as to obtain a perfectly flat band in TM polarization at low power (Fig. 2b).

### C Calculation of the condensation modes

For calculating the trajectory of the complex eigenfrequencies in Figs. 2f,l the parameters of $\mathcal{H}_{\mathrm{Lieb}}$ are kept constant and the evolution with pump power is completely driven by the "active" part of Eq. (1), parametrized by a single parameter $P$, equal to the total pump power. The finite size of the pump spot (Gaussian with intensity FWHM of 12 unit cells) is accounted for in the simulations (encoded in the specific functional form of the coefficients pump overlap coefficients $f_{lj}$). The decay rates of the polaritons are modeled as pillar specific in the tight-binding model, which are 50 $\mu$eV on B and C pillars and 60 $\mu$eV on A pillars. The motivation to make the latter larger by 20 % is due to the larger sidewall area of A pillars, which increases its exposure to the environment. As in the experiment, the 1D Lieb lattice simulated consists of 41 unit cells (123 pillars), with the blueshift to gain ratio $2g_R/R \approx 2.2$ extracted from the experimental data. Photonic disorder is included as a Gaussian distribution of the site energies of standard deviation 30 $\mu$eV, as estimated from the experiment (see section II B 3).

We show below examples of mode profiles calculated using this method. Fig. S1 shows the eigenmode of Eq. (1) with the lowest condensation threshold in the flat band (left column) and in the upper dispersive band (right column) [when pumping the lattice asymmetrically and symmetrically, respectively, see Fig. 2 of the main text]. Each line corresponds to a different realization of

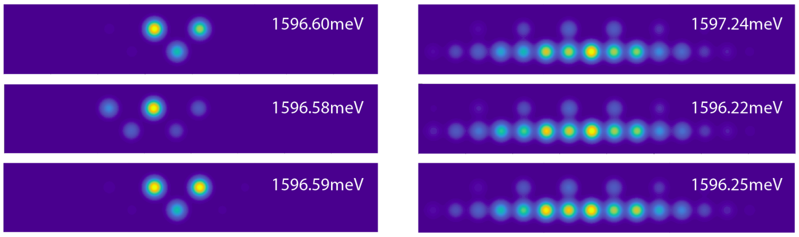


Figure S1. Calculated mode with lowest condensation threshold in the flat band (left column) and in the upper dispersive band (right column), when pumping the lattice with a spot covering 12 unit cells (intensity FWHM). Each line corresponds to a different realization of disorder.

disorder (drawn from a Gaussian distribution of standard deviation 30 $\mu$eV in the on-site energies). Flat band modes are localized, in contrast to upper band modes which are extended. Here the FWHM of the pump profile is taken to be 12 unit cells, which corresponds to the experimental condition and is much longer than the localization length of the flat band modes. Similar behaviors take place if we increase the FWHM of the pump to 24 unit cells, as shown in Fig. S2. The localization length in the flat band is barely affected, which shows that the localization is not due to the size of the pump. The extension of the dispersive band modes do appear to be wider.

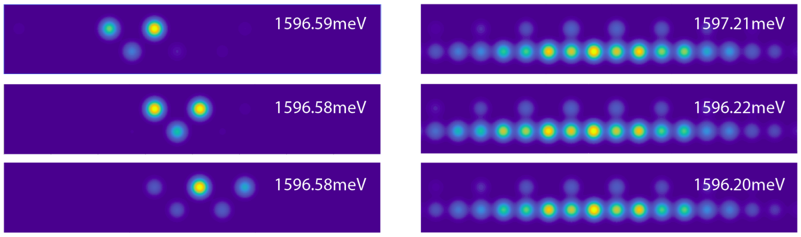


Figure S2. Same calculation as Fig. S1 but using a pump of 24 unit cells.

## D Calculation of the participation ratio

The calculation of the half participation ratio *HPR* in Fig. 3h relies on a direct diagonalization of the Hamiltonian, in presence of Gaussian disorder in the on-site energies (diagonal disorder):

- For the passive calculation based on $\mathcal{H}_{\text{Lieb}}$ (solid lines), the energy eigenvalues and associated participation ratios (as calculated from the corresponding eigenstates) are cast into bins and the disorder averaged *HPR* is obtained at a given energy by averaging within each bin. For each set of parameters we increase the lattice size $N$ as well as the number of disorder realizations until convergence is reached. In the same way we obtain the standard deviation.

- For the active calculation based on $\mathcal{H}(P)$ [Eq. (1)] (dots in Fig. 3h), the *HPR* in the flat band is averaged over the five flat band modes with the lowest thresholds in each numerical sample, and 1000 numerical samples are used. The parameters of the simulations are identical to those used in Figs. 2j,l (see section I C above).

# II. SUPPLEMENTARY EXPERIMENTAL DATA AND ANALYSIS

## A Condensation process

### 1. *Band structure versus pump power*

To describe the condensation process, in Fig. 2 of the main text, we focused on the polarization in which the condensation of interest is occurring: this is polarization TM for the upper dispersive band (left column of Fig. 2), and polarization TE for the flat band (right column). For completeness we present here data in both polarizations, for both excitation schemes, symmetric and antisymmetric.

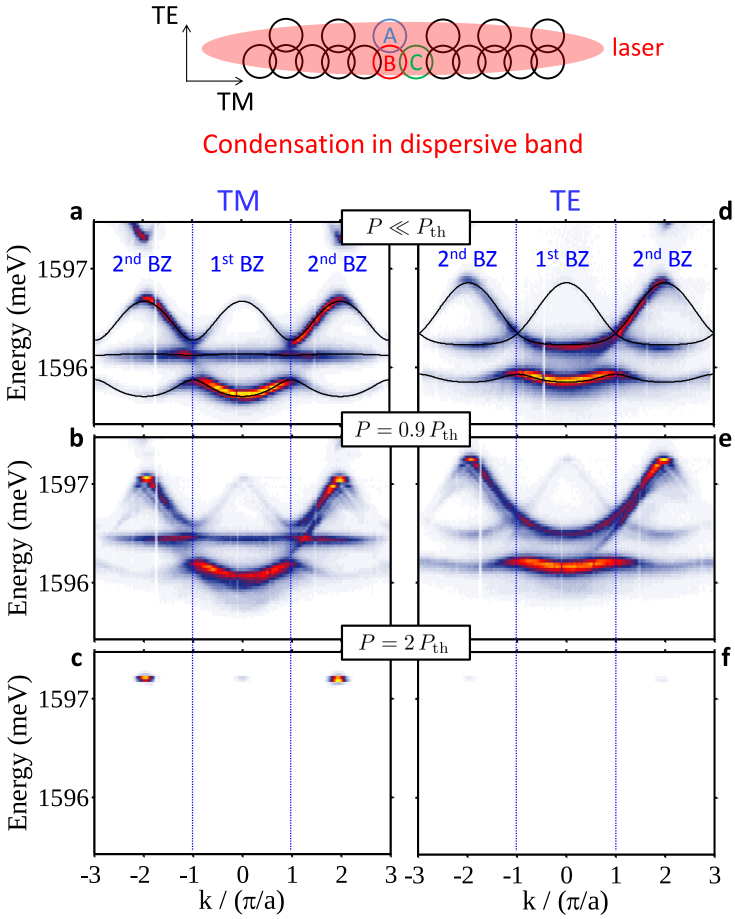


Figure S3. **Condensation in the dispersive band**, occurring when the pump is centered symmetrically on the lattice, as sketched in the top panel. The two columns, corresponding to the two polarizations TM and TE, monitor the momentum space emission when increasing the pump power from $P = 0.05\,P_{\mathrm{th}}$ to $P = 2\,P_{\mathrm{th}}$, where $P_{\mathrm{th}} = 4$ mW is the threshold power for this condensation process. For this spatial configuration of the pump, the band structure remains essentially unchanged for each polarization, subject only to an overall blueshift. The color scale is normalized to the maximum intensity within each row (corresponding to a fixed pump power).

Figure S3 shows the measured band structure when the pump is centered symmetrically on the lattice, as sketched in the top panel. The two columns, corresponding to the two polarizations TM and TE (see definition on the top panel), monitor the momentum space emission when increasing

the pump power from $P = 0.05\,P_{\rm th}$ to $P = 2\,P_{\rm th}$, where $P_{\rm th} = 4$ mW is the threshold power for this condensation process. The color code is normalized to the maximum intensity inside each panel.

As stated in the main text, for this spatial configuration of the pump the band structure remains essentially unchanged, in each polarization, and subject only to an overall blueshift due to the interaction with the excitonic reservoir. Condensation eventually occurs in the upper dispersive band in TM polarization, as seen in Fig. S3c. The emission is concentrated at the center of the Brillouin zones ($k = \pm 2\pi/a$ and $k = 0$), but the emission at $k = 0$ is strongly attenuated by a destructive interference in the far field[2,3]. For the same pump power in TE polarization (Fig S3f), the emission intensity is several orders of magnitude smaller (Fig S3c,f are plotted with the same color scale) as it remains in the linear (uncondensed) regime.

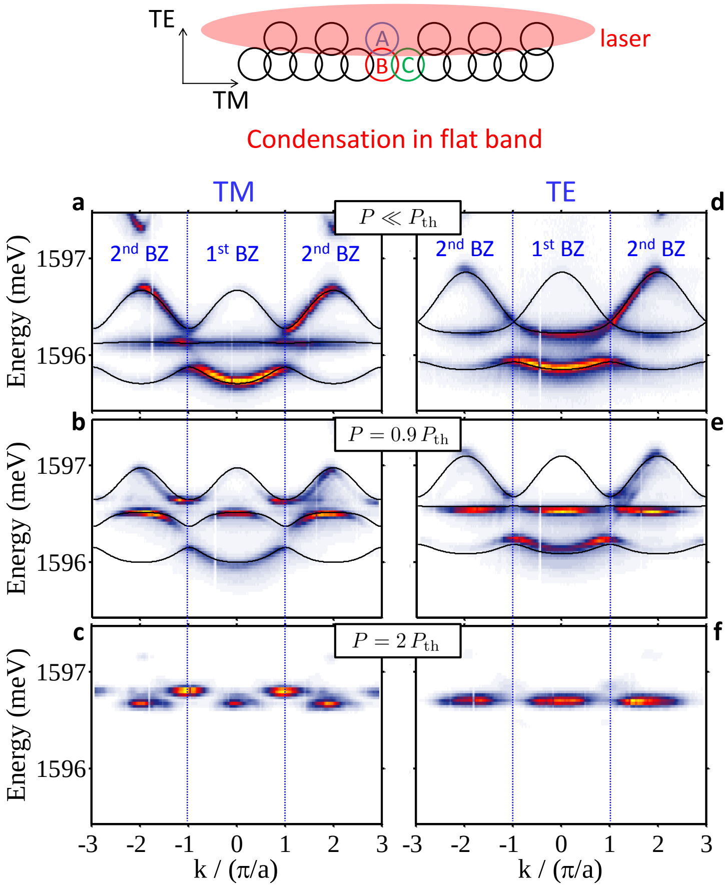


Figure S4. **Condensation in the flat band**, occurring when the pump is set to excite favorably pillars of type A, as sketched in the top panel. The two columns, corresponding to the two polarizations TM and TE, monitor the momentum space emission when increasing the pump power from $P = 0.05\,P_{\rm th}$ to $P = 2\,P_{\rm th}$, where $P_{\rm th} = 5$ mW is the threshold power for this condensation process. For this spatial configuration of the pump, pillars A develop a higher blueshift than other pillars, which reshapes the band structure with increasing pump power. The color scale is normalized to the maximum intensity for each pump power within each row (corresponding to a fixed pump power).

Figure S4 shows the measured band structure when the pump is set to excite favorably pillars of type A (see top panel). Due to the asymmetric pumping, pillars A here develop a higher blueshift than other pillars, which reshapes the band structure with increasing pump power. In TM polarization this blueshift introduces a detuning between pillars A and C, which destroys the flat band (see the general properties of the 1D Lieb lattice given in the main text). In TE

polarization, this blueshift exactly compensates the initial photonic detuning between pillars A and C (due to the anisotropy in the confinement of the electromagnetic field), so that a gapped flat band appears (**e**). In TM polarization, condensation occurs (**c**) simultaneously at the center of the (now dispersive) middle band and at the edge ($k = \pm\pi/a$) of the upper band. In TE polarization (**f**), condensation occurs only in the middle band, which is now flat. In the main text we concentrated on this flat band condensate.

### *2. Emission intensity and linewidth versus pump power*

Fig. S5 shows the intensity (red) and linewidth (green) of the flat band emission as a function of the pump power (conditions of Fig. S4, right column). The intensity encounters a non-linear threshold at $P = P_{\mathrm{th}} = 5$ mW, indicating the onset of bosonic stimulation, and the linewidth narrows, indicating the build-up of temporal coherence. We observed similar behavior for condensation in the dispersive band (conditions of Fig. S3, left column). These trends are typical of polariton condensation and identical to that observed in unpatterned 2D cavities[1,4].

We also verified that the blueshift of the emission energy between $P \ll P_{\mathrm{th}}$ and $P = 2\,P_{\mathrm{th}}$ does not exceed 4% of the Rabi splitting (which is 15 meV), certifying that the system remains in the strong coupling regime in the explored range of excitation power[1,4].

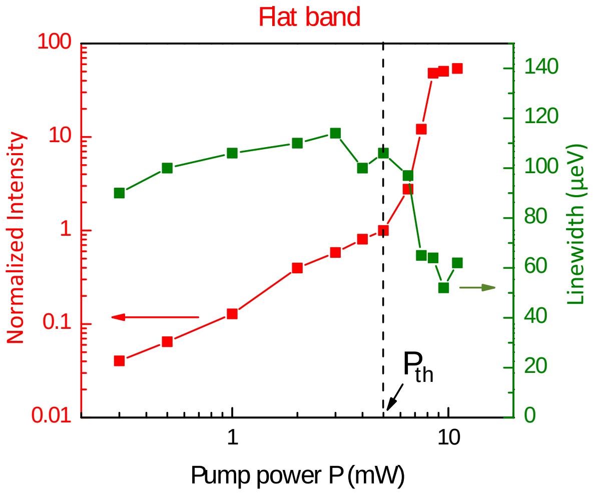


Figure S5. **Intensity and linewidth of the flat band emission** as a function of pump power. The characteristic features of polariton condensation are evidenced, with a strong non-linear increase of the intensity at threshold power $P = P_{\mathrm{th}}$, and a narrowing of the linewidth indicating the build-up of temporal coherence.

## B Properties of the condensates

In this section we present additional data on the physical properties of the condensates in both types of bands.

### 1. *Spatial map of the emission energy*

In Fig. 4 of the main text, we constructed a spatial map of the emission energy for both condensates (Fig. 4b and 4d). Fig. S6 presents the whole data used to obtain these maps. The power is set to $P = 2\,P_{\mathrm{th}}$ as for data shown in the main text.

Fig. S6a shows a real space image of the dispersive band condensate (same data as Fig. 2e of the main text). We used a spectrometer slit to select a narrow line of the emission (marked by the horizontal arrow), and disperse it in energy. The result is shown in **b**: the emission is monochromatic over the whole condensate within the experimental resolution (30 $\mu$eV). Fig. S6**c-e** shows the same measurements carried out on the flat band condensate (**c**). Here we separately analyzed both lines of pillars (cuts 1 and 2, indicated by the arrows). As seen in **d-e**, the emission energy shows a significant spatial inhomogeneity, in strong contrast with **b**. This allows one to directly visualize the localized flat band condensates, as shown in Fig. 4**b** of the main text.

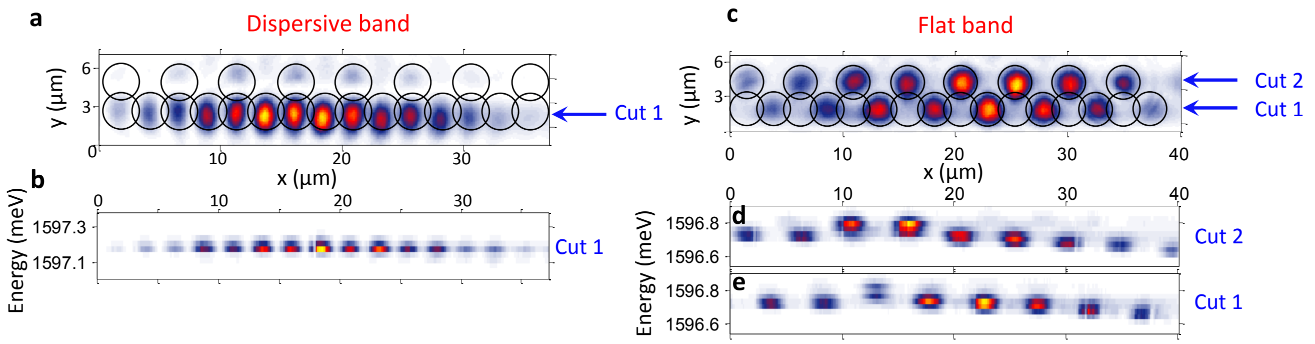


Figure S6. **Spatially-resolved measurements** carried out on the dispersive (left) and flat band (right) condensates at $P = 2\,P_{\mathrm{th}}$. **a**, Real space image of a dispersive band condensate; we use a spectrometer slit to select a narrow line of the emission (along the horizontal arrow), and disperse it in energy. The result is shown in **b**. **c-e**, Same measurements carried out on the flat band condensate (**c**). Here we successively analyze the two lines of pillars (cuts 1 and 2 indicated by the arrows).

### 2. *Phase structure of the condensates*

The phase structure of both types of condensates can by extracted by interferometry. For this we magnify the emission of one pillar (see arrow in Figs. S7**a** and **c**) of the condensate, to provide a flat phase reference, and make it interfere with the neighboring pillars. The resulting interferogram is shown on figure S7**b** for the case of the dispersive band condensate. At the intersection between two adjacent pillars, the fringes are shifted by half a period, indicating a $\pi$ phase shift: This is in agreement with the antisymmetric character of the upper band.

Fig. S7**c-d** show the same measurements carried out for the flat band condensate. The interferogram **d** also reveals a $\pi$ phase shift between bright pillars, in agreement with the structure of plaquette states, which have opposite phase on each pillar as depicted in Fig. 1b of the main text (gray). Note that any constructive superposition of plaquette-states (giving eigenstates of size 2 plaquettes, etc.) has the same phase structure.

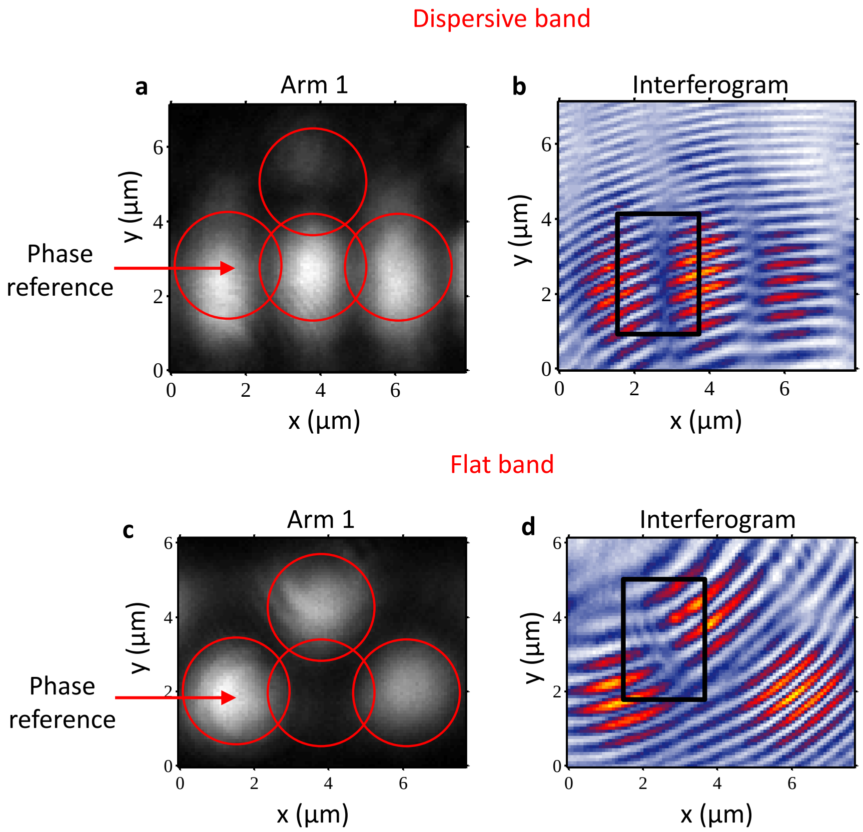


Figure S7. **Phase structure of the condensates** of dispersive (top row) and flat band (bottom row). **a-b**, The emission of one pillar (indicated by the arrow in **a**) of the dispersive band condensate is magnified, and overlapped with its neighboring pillars (image **a**) to produce the interferogram **b**. A $\pi$ phase shift (see black rectangle) of the fringes appears between adjacent pillars, in agreement with the antisymmetric character of the upper band. **c-d**, Same procedure carried out for the flat band condensate. The interferogram **d** also reveals a $\pi$ phase shift between bright pillars, in agreement with the structure of plaquette-states.

### *3. Estimation of disorder strength in our samples*

In our lattices, the strength of diagonal disorder can be estimated from the energy distribution of flat band condensates, as given by Fig. 4b of the main text and similar data obtained on different disorder realizations. The standard deviation is 30 $\mu$eV, representing $\sim 2\%$ of the on-site energy of the micropillars (photonic confinement energy), corresponding to a fluctuation of about 1% of the micropillar radius around its nominal value.

### *4. Effect of diagonal Vs. non-diagonal disorder in the flat band*

In the calculation of the participation ratio (Fig. 3h) we considered diagonal disorder (i.e. on the on-site energies) only, as the flat band is robust to non-diagonal disorder (i.e. on the tunnel couplings)[5]. This is confirmed by Fig. S8, comparing the half participation ratio *HPR* calculated from $\mathcal{H}_{\text{Lieb}}$ for three situations:

- as a function of diagonal disorder, at zero non-diagonal disorder (red plain line, corresponding

to the data of Fig. 3h in the main text);

- as a function of non-diagonal disorder, at zero diagonal disorder (red dotted line);
- as a function of diagonal disorder, at 30 $\mu$eV non-diagonal disorder (blue plain line).

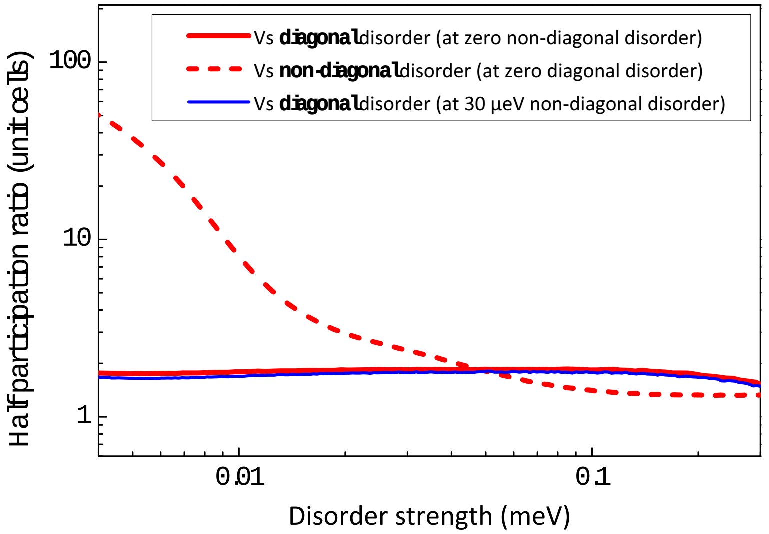


Figure S8. Calculated half participation ratio *HPR* as a function of the disorder strength in the flat band.

We observe that the amount of non-diagonal disorder needed to reproduce the experimental *HPR* ($\sim 2$ unit cells) is 40 $\mu$eV (it would diverge in the limit of a perfect flat band). This value, which represents 20 % of the tunnel couplings is unrealistic given the quality of the technological process (fluctuations of the confinement energies are of order 2 % only). On the other hand, an amount of 3 $\mu$eV only of diagonal disorder (corresponding to the bandwidth of the flat band) is sufficient to saturate the participation ratio down to $\sim 2$ unit cells.

This confirms that the dominant effect on the localization in the flat band is diagonal disorder. As a final check, we calculate the participation ratio as a function of diagonal disorder, at a fixed strong non-diagonal disorder of 30 $\mu$eV (blue line): the effect of adding non-diagonal disorder is negligible as diagonal disorder very quickly saturates the participation ratio to a very low value.

### 5. *Estimation of polariton-polariton interactions*

In our experiments, polaritons encounter two types of interactions. First, each polariton interacts with the reservoir of excitons (see Eq. (1) in the main text), resulting in a modification of the band structure with the pump power, as discussed in the main text (Fig. 2). Second, polaritons mutually interact within the condensate, yielding a cubic (Kerr) nonlinearity.

We estimate this polariton-polariton interaction energy to be of order 0.1 $\mu$eV in our experiments, thus much smaller than disorder (30 $\mu$eV) and dissipation (50 $\mu$eV). We here detail the estimation of this interaction energy.

The polariton-polariton (Kerr-type) interaction energy reads $NU$, where $N$ is the number of polaritons in the condensate and $U$ is the single-polariton non-linearity, which can be estimated by[6] $U = (g \cdot X^4)/(N_{\mathrm{QW}} \cdot \mathcal{A})$. Here, $g \sim 10\ \mu\mathrm{eV} \cdot \mu\mathrm{m}^2$ is the 2D exciton-exciton interaction constant[6,7], $X = 0.64$ is the excitonic weight of the polariton wavefunction in our experiments, $N_{\mathrm{QW}} = 12$ is

the number of quantum wells and $\mathcal{A} \simeq 80\ \mu\mathrm{m}^2$ is the area of the condensate at half maximum. This yields $U \sim 0.002\ \mu$eV. The polariton population $N$, estimated by the ratio between the emission intensity of the condensate ($P = 2\,P_{\mathrm{th}}$) and the intensity at threshold ($P = P_{\mathrm{th}}$), is $N \sim 50$ according to Fig. S5. This yields an interaction energy $NU \sim 0.1\ \mu$eV.

To achieve higher interaction energies (up to $\sim 1$ meV)[8], resonant pumping can be used to inject a much higher polariton population $N$. This should allow studying the interplay of disorder and interactions in the flat band, and potentially realize strongly correlated phases of polaritons[9–11].

Here the maximum interaction energy that can be investigated, while stile keeping the flat band isolated from other bands, is set by the gap between the flat band and the upper dispersive band ($\sim 150\ \mu$eV). This value overcomes both disorder and dissipation, and should thus already produce a regime qualitatively different from the one studied in the article. To investigate even higher interaction energies, the lattice structure can be further engineered to increase the gap to the upper band. For this the flat band could be intentionally redshifted inside the gap for instance by blueshifting pillars B (e.g. by reducing their radius), or alternatively, the tunnel coupling could be increased by reducing the separation between pillars in the lattice.

### 6. *Stability of flat band condensates*

We here investigate the stability of flat band condensates.[12–14] For completeness we add to Hamiltonian $\mathcal{H}(P)$ [Eq. (1)] a cubic nonlinear term corresponding to polariton-polariton interactions (see section II B 5), despite its low order of magnitude compared to other energy scales in the experiment.

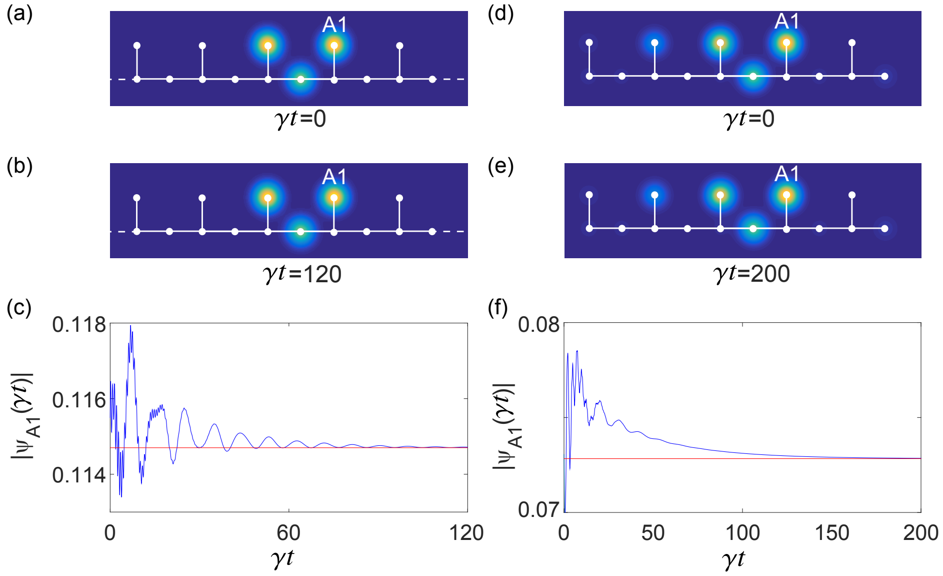


Figure S9. **Stability of flat band condensates. a**, Calculated stationary spatial profile of a typical flat band mode in the conditions of the experiments (lattice length 41 unit cells). **b**, Calculated profile at time $\gamma t = 120$ (where $\gamma = 50\ \mu$eV is the polariton decay rate) after perturbing all lattice sites at $t = 0$. **c**, Time evolution of the wavefunction amplitude on site A1 (see panel a). **d-f**, Similar simulations carried out for a lattice of 5 unit cells.

We simulate the transient behavior of a flat band mode a few percent above its condensation threshold (the analysis at high pump powers deals with multi-mode effects, which is beyond the

scope of the present work). As shown in Fig. S9, we first calculate the stationary solution of a flat band mode just above its threshold using a time-independent method[15]. In this example the system is the same as that used in Figs. 2f,l in the manuscript with 41 unit cells, and the stationary mode is highly localized and represents a plaquette state (see panel a). We then perturb its wavefunction on all lattice sites by adding a white noise and simulate the transient behavior of this mode. Panel c shows its amplitude as a function of time on lattice site A1, and it is clear that the perturbed wavefunction converges to the stationary state (panel b shows the mode pattern at long time delays). $\gamma$ in panel c is the polariton decay rate, taken as 50 $\mu$eV (with $\hbar = 1$). This behavior is consistent as we vary the pump power or change the number of unit cells (see panels d-f showing similar simulations for a system with 5 unit cells). This analysis suggests that the flat band modes observed in the experiment are stable.

.

---

* Now at Laboratoire Kastler Brossel, Université Pierre et Marie Curie, 75005 Paris, France.

1 Kasprzak, J. *et al.* Bose–Einstein condensation of exciton polaritons. *Nature* **443**, 409–414 (2006).

2 Shirley, E. L., Terminello, L. J., Santoni, A. & Himpsel, F. J. Brillouin-zone-selection effects in graphite photoelectron angular distributions. *Phys. Rev. B* **51**, 13614–13622 (1995). URL http://link.aps.org/doi/10.1103/PhysRevB.51.13614.

3 Jacqmin, T. *et al.* Direct observation of dirac cones and a flatband in a honeycomb lattice for polaritons. *Phys. Rev. Lett.* **112**, 116402 (2014).

4 Carusotto, I. & Ciuti, C. Quantum fluids of light. *Rev. Mod. Phys.* **85**, 299–366 (2013). URL http://link.aps.org/doi/10.1103/RevModPhys.85.299.

5 Mukherjee, S. *et al.* Observation of a localized flat-band state in a photonic lieb lattice. *Phys. Rev. Lett.* **114**, 245504 (2015). URL http://link.aps.org/doi/10.1103/PhysRevLett.114.245504.

6 Ciuti, C., Savona, V., Piermarocchi, C., Quattropani, A. & Schwendimann, P. Role of the exchange of carriers in elastic exciton-exciton scattering in quantum wells. *Phys. Rev. B* **58**, 7926–7933 (1998). URL http://link.aps.org/doi/10.1103/PhysRevB.58.7926.

7 Ferrier, L. *et al.* Interactions in confined polariton condensates. *Phys. Rev. Lett.* **106**, 126401 (2011). URL http://link.aps.org/doi/10.1103/PhysRevLett.106.126401.

8 Abbarchi, M. *et al.* Macroscopic quantum self-trapping and Josephson oscillations of exciton polaritons. *Nature Physics* **9**, 275–279 (2012).

9 Huber, S. D. & Altman, E. Bose condensation in flat bands. *Phys. Rev. B* **82**, 184502 (2010). URL http://link.aps.org/doi/10.1103/PhysRevB.82.184502.

10 Wu, C., Bergman, D., Balents, L. & Das Sarma, S. Flat bands and Wigner crystallization in the honeycomb optical lattice. *Phys. Rev. Lett.* **99**, 070401 (2007). URL http://link.aps.org/doi/10.1103/PhysRevLett.99.070401.

11 Biondi, M., van Nieuwenburg, E. P. L., Blatter, G., Huber, S. D. & Schmidt, S. Incompressible polaritons in a flat band. *Phys. Rev. Lett.* **115**, 143601 (2015). URL http://link.aps.org/doi/10.1103/PhysRevLett.115.143601.

12 Vicencio, R. A. & Johansson, M. Discrete flat-band solitons in the kagome lattice. *Phys. Rev. A* **87**, 061803 (2013). URL http://link.aps.org/doi/10.1103/PhysRevA.87.061803.

13 Molina, M. I. Localized modes in nonlinear photonic kagome nanoribbons. *Phys. Lett. A* **376**, 3458–3461 (2012).

14 Leykam, D., Flach, S., Bahat-Treidel, O. & Desyatnikov, A. S. Flat band states: Disorder and nonlinearity. *Phys. Rev. B* **88**, 224203 (2013). URL http://link.aps.org/doi/10.1103/PhysRevB.88.224203.

[15] Ge, L., Nersisyan, A., Oztop, B. & Tureci, H. E. Pattern formation and strong nonlinear interactions in exciton-polariton condensates. *arXiv:1311.4847* (2013).
